# Supplementary material for: Towards Looped Models Done Right, Part II: Rethinking at Fixed Points
Source: arXiv:2610.06833 source file (2026-10-05)
Supplement: Supplementary file 1 [file injection_switch_loss_figure.tex]

\begin{figure}[!htbp]
\centering
\includegraphics[width=\linewidth]{figures/appendix/injection_switch_loss.pdf}
\caption{\textbf{Both switches lower late-training loss.} Training CE of the four cells of Table~\ref{tab:orthoinj-normalization-init} over the final $20\%$ of training, as a $512$-step rolling median. All cells see the same sampled depths.}
\label{fig:injection-switch-loss}
\end{figure}
