# Supplementary material for: Towards Looped Models Done Right, Part II: Rethinking at Fixed Points
Source: arXiv:2610.06833 source file (2026-10-05)
Supplement: Supplementary file 2 [file orthoinj_switch_2x2.tex]

\begin{table}[!htbp]
\centering\resulttablestyle
\caption{\textbf{Dropping prelude RMSNorm and projecting the carryover each lower perplexity, and their gains add up.} S models trained with PLN-5 and evaluated at $R=5$ without KV reuse. Norm is prelude RMSNorm and Proj.\ the carryover projection; LR is each cell's own selected learning rate; Sel.\ is PPL on the LR-selection set; AVG is the seven-task mean of Table~\ref{tab:architecture-fullkv}.}
\label{tab:orthoinj-normalization-init}
\renewcommand{\arraystretch}{\resultrowstretch}
\begin{NiceTabular}{@{\hspace{6pt}}lccccccc@{\hspace{6pt}}}
\CodeBefore
\rowcolor{papergray}{3}
\Body
\toprule
\multicolumn{4}{c}{Training} & \multicolumn{3}{c}{PPL $\downarrow$} & Down.\ (\%) $\uparrow$ \\
\cmidrule(lr){1-4}\cmidrule(lr){5-7}\cmidrule(lr){8-8}
Recipe & Norm & Proj. & LR & Sel. & Val. & Wiki & AVG \\
\midrule
\multicolumn{8}{l}{\textbf{S scale: (100M, 21.5B tokens)}} \\
Parcae-Decay & \checkmark &  & $0.0015$ & 6.86 & 6.71 & 21.24 & 41.35 \\
$+$ projection & \checkmark & \checkmark & $0.0015$ & 6.84 & 6.67 & 21.26 & 41.37 \\
$-$ prelude norm &  &  & $0.002$ & 6.79 & 6.63 & \textbf{21.14} & 41.34 \\
OrthoInj ($-$norm $+$proj.) &  & \checkmark & $0.002$ & \textbf{6.78} & \textbf{6.60} & 21.16 & \textbf{41.59} \\
\bottomrule
\CodeAfter
\begin{tikzpicture}
\foreach \sepcol in {5,8}{
\draw[draw=resultgrouprule,line width=0.35pt] (1-|\sepcol) -- (3-|\sepcol);
\draw[draw=resultgrouprule,line width=0.35pt] (4-|\sepcol) -- (8-|\sepcol);
}
\end{tikzpicture}
\end{NiceTabular}
\end{table}
